# Supplementary material for: VIPER: Volume Invariant Position-based Elastic Rods
Source: arXiv:1906.05260 source file (2019-06-12)
Supplement: Supplementary file 1 [file appendix_collision.tex]

\section{Collision resolution}
\AT{Is this section still needed?}
\begin{draft}
The corrections are given by: \TODO{missing $h^2$ for now} \TODO{find better than $\alpha$ for compliance}
\begin{equation}
    \Delta \lambda = \frac{C(x) - \alpha \lambda}{(w^a_1 + \omega^a_1) \alpha_1^2 + (w^a_2 + \omega^a_2) \alpha_2^2 + (w^b_1 + \omega^b_1) \beta_1^2 + (w^b_2 + \omega^b_2) \beta_2^2 + \alpha}
\end{equation}
\begin{align}
    \Delta p^a_1 &=  h^2 \alpha_1 w^a_1 \frac{p_a(u) - p_b(v)}{\lVert p_a(u) - p_b(v) \rVert} \Delta \lambda \\
    \Delta p^a_2 &=  h^2 \alpha_2 w^a_2 \frac{p_a(u) - p_b(v)}{\lVert p_a(u) - p_b(v) \rVert} \Delta \lambda \\
    \Delta p^b_1 &= -h^2 \beta_1 w^b_1 \frac{p_a(u) - p_b(v)}{\lVert p_a(u) - p_b(v) \rVert} \Delta \lambda \\
    \Delta p^b_2 &= -h^2 \beta_2 w^b_2 \frac{p_a(u) - p_b(v)}{\lVert p_a(u) - p_b(v) \rVert} \Delta \lambda \\
    \Delta r^a_1 &=  h^2 \alpha_1 \omega^a_1 \Delta \lambda \\
    \Delta r^a_2 &=  h^2 \alpha_2 \omega^a_2 \Delta \lambda \\
    \Delta r^b_1 &=  h^2 \beta_1 \omega^b_1 \Delta \lambda \\
    \Delta r^b_2 &=  h^2 \beta_2 \omega^b_2 \Delta \lambda
\end{align}
\end{draft}
